# Supplementary material for: Is there a polaron signature in angle-resolved photoemission of CsPbBr3?
Source: arXiv:2203.15070 ancillary file (2022-06-28)
Supplement: Supplementary file 1 [file Sajedi_Supplement.pdf]

# Is there a polaron signature in angle-resolved photoemission of CsPbBr<sub>3</sub>?

Maryam Sajedi,<sup>1,2</sup> Maxim Krivenkov,<sup>1</sup> Dmitry Marchenko,<sup>1</sup> Jaime Sánchez-Barriga,<sup>1</sup> Anoop K. Chandran,<sup>3,4</sup> Andrei Varykhalov,<sup>1</sup> Emile D. L. Rienks,<sup>1</sup> Irene Aguilera,<sup>5,\*</sup>, Stefan Blügel,<sup>3</sup> Oliver Rader<sup>1</sup>

<sup>1</sup> *Helmholtz-Zentrum Berlin für Materialien und Energie,  
Albert-Einstein-Str. 15, 12489 Berlin, Germany*

<sup>2</sup> *Institut für Physik und Astronomie, Universität Potsdam,  
Karl-Liebknecht-Str. 24/25, 14476 Potsdam, Germany*

<sup>3</sup> *Peter Grünberg Institut and Institute for Advanced Simulation,  
Forschungszentrum Jülich and JARA, 52425, Jülich Germany*

<sup>4</sup> *Department of Physics, RWTH Aachen University, 52056 Aachen Germany and*

<sup>5</sup> *Institute of Energy and Climate Research, IEK-5 Photovoltaics,  
Forschungszentrum Jülich, 52425 Jülich, Germany*

## REPRODUCIBILITY OF ARPES RESULTS

Figures S 1 and S 2 demonstrate the reproducibility of the ARPES experiments on CsPbBr<sub>3</sub>, with regard to effective mass and determination of the high symmetry points, respectively. Fig. S 1(a)–S 1(d) Shows the valence band maximum along the X-R direction for three different CsPbBr<sub>3</sub> crystals. The hole effective masses estimated from the four different measurements are in the range between 0.19 and 0.23  $m_0$  with an average of 0.203  $m_0$ .

In order to reassure the determination of high symmetry points, we have conducted systematic photon energy dependent measurements for two CsPbBr<sub>3</sub> crystals. Fig. S 2 shows the second derivative of intensity plots along  $M-R-M-R$  extracted from two sets of  $k_{\perp}$  dependent measurements taken with S 2(a) linear horizontal, and S 2(b) and S 2(c) circularly polarized light. The plots of ARPES intensity ( $k_{\perp}$ ,  $k_{\parallel}$ ) in Fig. S 2 (a) are taken with photon energies between 21 and 83 eV, with 2 eV steps, unveiling  $R$  point dispersions around  $\mathbf{k}_{\perp} = 2.61$  ( $h\nu = 29$  eV) and  $3.66 \text{ \AA}^{-1}$  ( $h\nu = 54$  eV). Plots of binding energy versus photon energy Fig. S 2(b) and  $\mathbf{k}_{\perp}$  Fig. S 2(c) are provided with photon energies between 14 and 43 eV, with 1 eV step, which verify the assignment of 19, 29, and 39 eV to the high symmetry points  $M$ ,  $R$ , and  $M$ , respectively.

## EFFECTIVE MASS AND BAND GAP

The behavior of the theoretically predicted effective mass versus band gap is exhibited in Fig. S 3, in which the results of different band calculation methods found in the literature have been extracted and compared with our  $GW$  calculations. As it can be seen, generally the effective mass increases in systems with larger band gaps.

## THEORETICAL METHODS

Our calculations were carried out with the DFT code FLEUR [36] and the  $GW$  code SPEX [37], both based on the all-electron FLAPW formalism. The spherical harmonics expansion of the LAPW basis includes functions up to an angular momentum cutoff  $l_{max} = 10$  within the muffin-tin spheres and includes all basis functions with plane-wave vectors smaller than  $3.6 \text{ Bohr}^{-1}$ . For the DFT calculations, we employ the Perdew-Burke-Ernzerhof (PBE) [40] parametrization of the generalized gradient approximation (GGA). We use computationally determined lattice constants consistent with exchange-correlation potential. Based on the observation of a community effort benchmarking different electronic structure methods [44] that the lattice constants determined by the main codes differ by less than 1%, we decided to adopt the lattice constants from the Materials Projects database [45, 46] determined by the VASP code. For the cubic lattice, we use the lattice parameter of  $6.0173 \text{ \AA}$  of [46]. For the orthorhombic one, we use lattice constants of  $a = 8.3704$ ,  $b = 8.4253$ , and  $c = 12.0113 \text{ \AA}$  extracted from [45]. These lattice constants are about 2% larger for the cubic structure and about 1.3% larger for the orthorhombic one compared

---

\* Present address: Institute of Physics, University of Amsterdam, Netherlands.

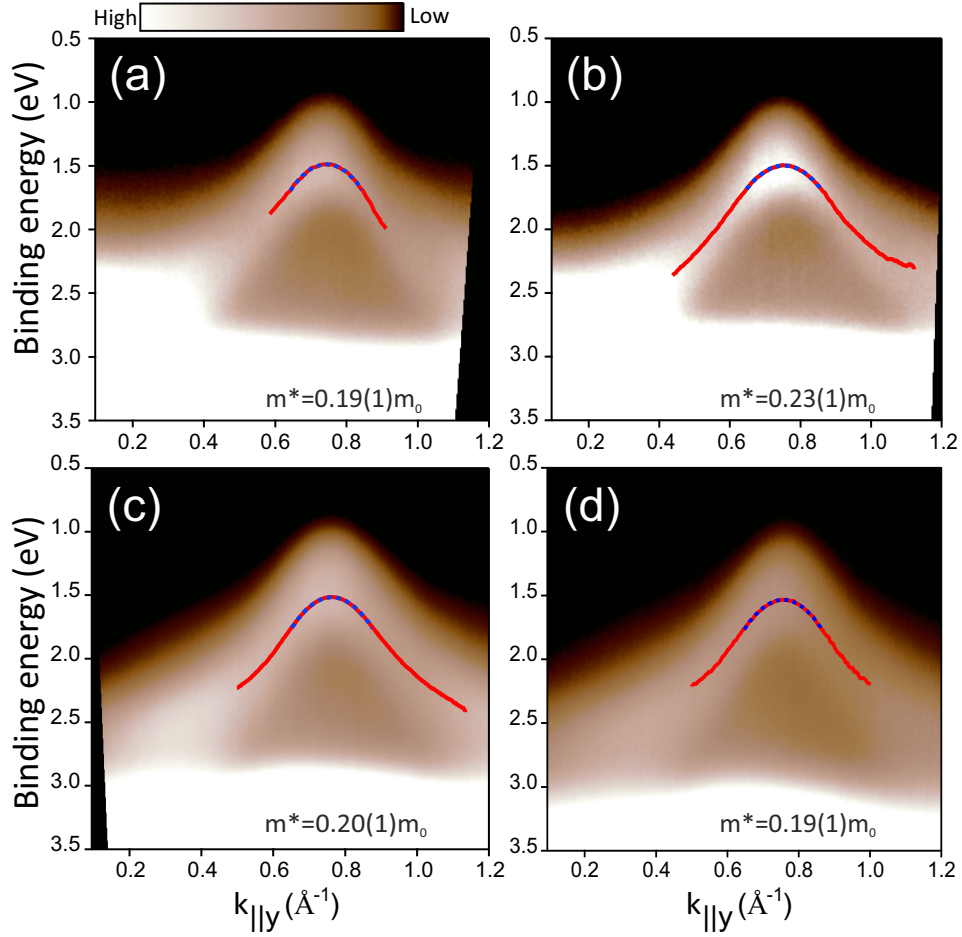

Fig. S 1. Topmost band dispersion at room temperature for three different samples, taken with 29 eV photon energy. (c) and (d) are from the same sample but different spots on the surface. The red and blue lines indicate the Gaussian fits on the dispersions and the parabola fits of the peaks, respectively.

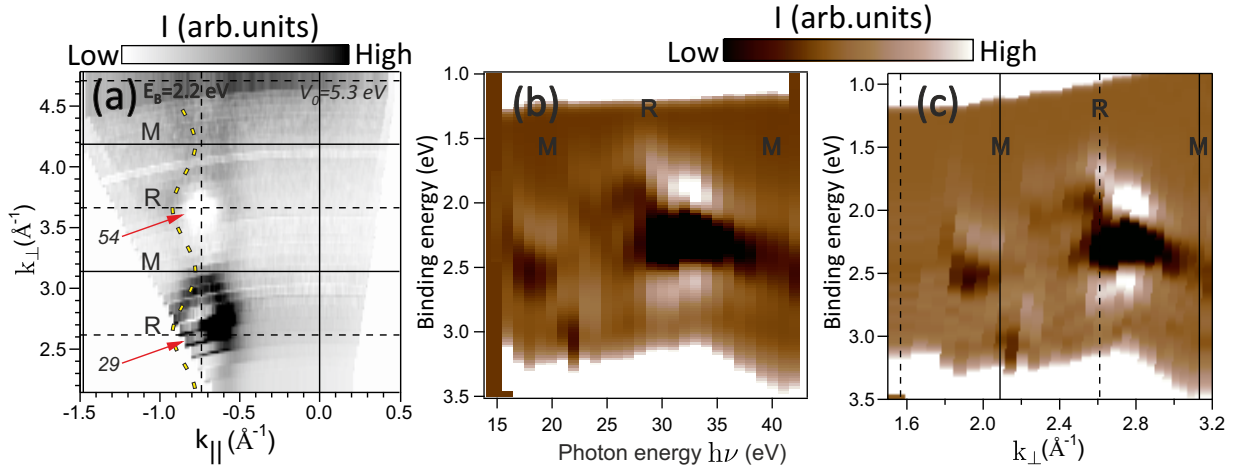

Fig. S 2. Valence band maximum determination via ARPES photon energy dependent measurements. (a) Cut through the path M-R-M-R converted to momentum ( $k_{\perp}$ ,  $k_{\parallel}$ ) space, corresponding to the second derivative of intensity in Fig. 2(e). (b) Second derivative  $k_{\perp}$  dependent measurements using a database circularly polarized light along the  $\bar{\Gamma} - \bar{M}$  direction indicating high symmetry points at 19, 29, and 39 eV. (c) Conversion of (b) into perpendicular momentum space using  $V_0 = 5.3$  eV.

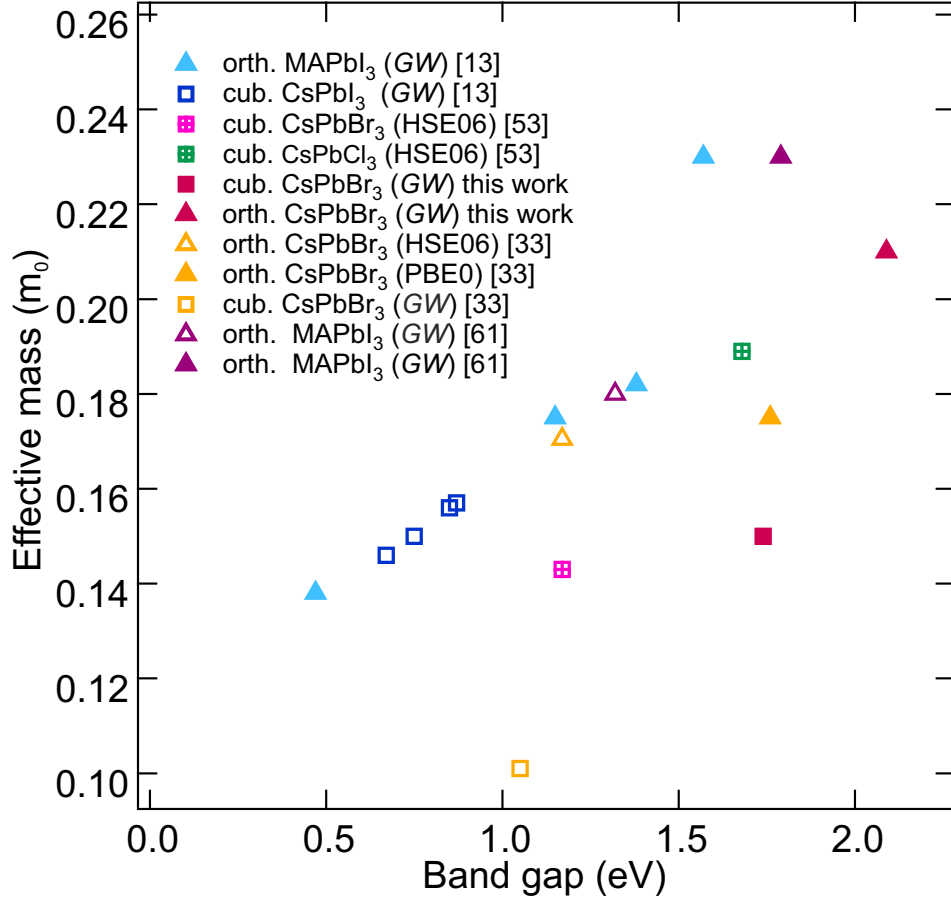

Fig. S 3. Hole effective mass versus band gap for several band structure calculations in the literature for various perovskites in comparison to our *GW* calculations. Values are extracted from Refs. [13], [33], [53], and [61].

to the experimental values extracted from powder X-ray diffraction patterns. A  $6 \times 6 \times 6$   $\mathbf{k}$  point grid is used to sample the Brillouin zone. In the spheres, relativistic effects are included in the scalar relativistic approximation [41], while the spin-orbit coupling (SOC) is incorporated self-consistently employing the “second variation” technique [42]. For the *GW* calculations, an angular momentum cutoff of  $l = 5$  and a plane-wave cutoff of  $2.7 \text{ Bohr}^{-1}$  are employed to construct the mixed product basis [37]. For the cubic structure, a  $4 \times 4 \times 4$   $\mathbf{k}$  point mesh and 300 bands are used. For the orthorhombic one, we use a  $3 \times 3 \times 3$   $\mathbf{k}$  point mesh and 1500 bands. Semi-core states Cs 5s, Cs 5p, Pb 5d, and Br 3d are treated as valence states by the use of local orbitals. The screened Coulomb interaction is calculated within the random-phase approximation without resorting to a plasmon-pole model for the frequency dependence. The frequency convolution of the self-energy is evaluated with the use of an analytic-continuation technique. For the interpolation of the band structures, we use maximally localized Wannier functions obtained by the WANNIER90 library [43].

#### GW VALENCE BAND CALCULATIONS (ORTHORHOMBIC)

Figure S 4(b)–S 4(g) represents the *GW* valence band structure calculations for the orthorhombic unit cell computed for six different crystallographic directions and including SOC. This figure reveals the valence bands and the anisotropy of the hole effective mass. Note that experiments were done with a synchrotron beam spot of size  $\sim 100 \mu\text{m}$ , therefore most of our ARPES results are average of all possible nonequivalent  $\Gamma - \text{M}$ -like directions ([010], [100] etc). We note that from our calculations the band gap at Gamma is 2.09 eV.

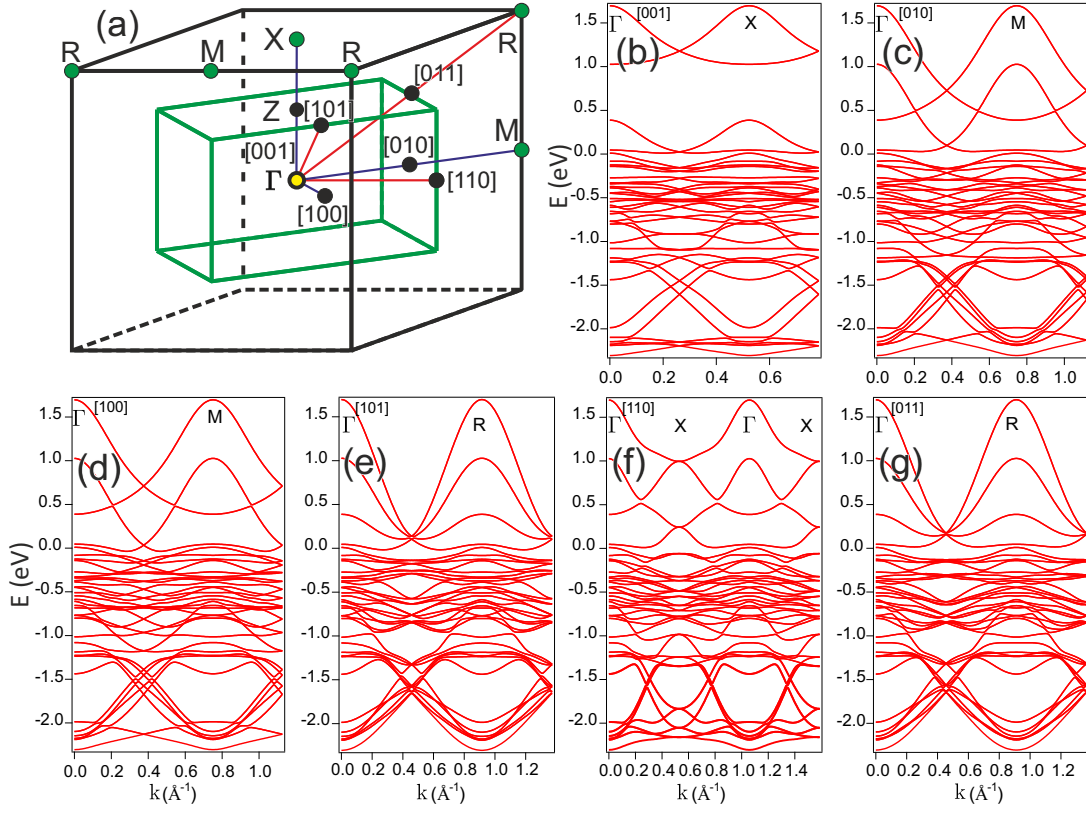

Fig. S 4. (a) Cubic and orthorhombic Brillouin zones. (b)–(g)  $GW$  valence band structure for 6 different crystallographic directions in the orthorhombic Brillouin zone, which are marked in (a). High-symmetry points are labeled in cubic notation to make comparison with experimental results easier.

## BENCHMARKING CALCULATIONS

Our  $GW$  band gap values for the cubic and the orthorhombic structures are 1.74 eV and 2.09 eV, respectively. We are aware of two other  $GW$  calculations for the cubic structure: that of Puppini *et al.* [33] (band gap 1.05 eV) and that of Wiktor *et al.* [54] (band gap 0.94 eV). All three  $GW$  results are obtained with perturbative one-shot  $GW$ , using the PBE functional of DFT as starting point, and with a full treatment of SOC.

The two values in the literature are significantly smaller than ours. To try to explain the origin of these differences, we have performed calculations with the parameters of the two references mentioned above. Increasing the mesh of  $\mathbf{k}$  points to  $6 \times 6 \times 6$  and the number of bands to 500 (to reproduce results from [33]), we obtain a band gap of 1.74 eV. Increasing the number of bands up to 2000 (while keeping the  $\mathbf{k}$ -mesh at  $4 \times 4 \times 4$  to reproduce results from [54]) leads to a band gap of 1.78 eV. Therefore, we are confident that our value of 1.74 eV is converged with respect to both  $\mathbf{k}$ -mesh and bands. Using the same lattice parameters of [33], we obtain a band gap of 1.59 eV. Therefore, the lattice parameters cannot explain the band gap differences with the previous literature.

There are however, other important differences between our calculations and the former ones: while [33] and [54] used the plane-waves pseudopotentials method and the plasmon-pole model for the  $GW$  calculations, we use the all-electron FLAPW method, and we perform a full frequency dependent integration for the calculation of the screened Coulomb interaction  $W$  instead of resorting to a plasmon-pole approximation.

To shed more light onto the comparison with previous values, we can also compare the DFT results that are used as the starting point for the  $GW$  calculations. Our DFT-PBE band gap without SOC is 1.81 eV. Puppini *et al.* do not provide the DFT-PBE value without SOC. Wiktor *et al.*, on the other hand, give a value of 1.54 eV. The latter calculation, as well as ours, are obtained using the lattice structure of the Materials Project database extracted from [46]. The value of the band gap reported in the database is 1.782 eV. Our value is in better agreement with this reference value than the one from Wiktor *et al.* and also closer to other values in the literature: 1.663 eV [55], 1.764 eV [56], 1.76 eV [57], and 1.75 eV [58].

When SOC is further added, the difference between our result and [33] and [54] increases. They report a PBE-SOC

band gap of 0.32 eV, whereas our value is 0.85 eV. They do not explain how the SOC is included in their calculations. In our case, it is included with an accurate self-consistent second-variation treatment. Other values in the literature tend to be in between: 0.54 eV [59], 0.61 eV [57], 0.64 eV [58].

### EFFECTIVE MASS CONVERGENCE

A careful analysis, similar to Ref. [33], has been done to determine the hole effective masses of both experimental and theoretical bands. Bands were fitted with a parabolic function in different angular momentum intervals ( $\Delta k$ ) around the high symmetry point. Figure S 5 demonstrates hole effective mass values as a function of  $\Delta k$  in decreasing trend, where we determine the effective mass. As a result, mass value of  $m_h^* = 0.19 m_0$  is determined for the topmost band in ARPES [Fig. S 5(a)]. From *GW* calculations, values of  $m_h^* = 0.15(2) m_0$  and  $0.20(2) m_0$  are obtained for cubic *R* and *M* points, respectively S 5(b). Corresponding *GW* masses for orthorhombic structure depend on the crystallographic axis and are in average  $m_h^* = 0.214 m_0$  and  $0.185 m_0$  for [001],  $0.212 m_0$  for [011],  $0.208 m_0$  for [101],  $0.223 m_0$  for [100],  $0.228 m_0$  for [110], and  $0.229 m_0$  for [010] (c). In the experiment, the effective mass is probed along the cubic *X-R* direction. This corresponds to the orthorhombic [010] [Fig. S 4(c)] and [100] [Fig. S 4(d)] directions because cubic *X* is projected on  $\Gamma$  and cubic *R* is projected on cubic *M*. The average of these two effective masses is  $0.226 m_0$ .

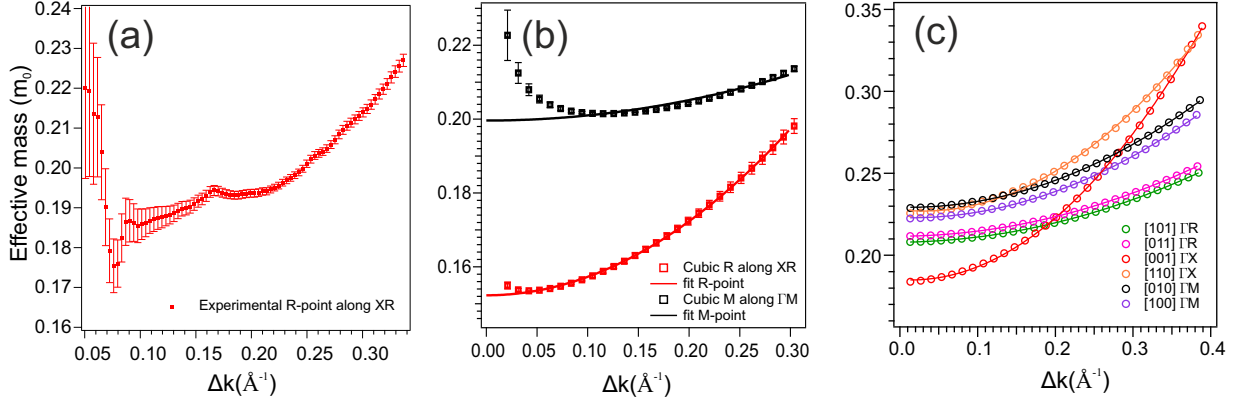

Fig. S 5. (a)–(c) Parabola fitting of the valence band maximum in the vicinity of the high symmetry points, up to the convergence of effective mass fit with a descending momentum interval. Vertical axes in the figures indicate the hole effective mass values times the free-electron mass ( $m_0$ ). Solid lines are fits. Effective mass convergence for (a) experimental *R* point along the *X* – *R* direction taken from ARPES spectra shown in Fig. 3(c), *GW* hole masses for (b) cubic *R* and *M* points from Fig. 1 (b) and Fig. 1(c), (c) six different directions in the orthorhombic Brillouin zone in Fig. S 4(b)–S 4(g).

In summary, the DFT band-gap values of [33] and [54] are significantly smaller than other values in the literature. The DFT starting point for their *GW* calculations is by 0.53 eV smaller than ours. Given the large difference in the starting point and in the methods used, it is not surprising that our *GW* value is by  $\sim 0.7 - 0.8$  eV larger.
